# Supplementary material for: Symmetry-driven embedding of networks in hyperbolic space
Source: arXiv:2406.10711 ancillary file (2025-04-24)
Supplement: Supplementary file 1 [file supplementary.pdf]

# Supplementary Information for
# Symmetry-driven embedding of networks in hyperbolic space

Simon Lizotte[1,2], Jean-Gabriel Young[1,3,4], Antoine Allard[1,2,4]

1. Département de physique, de génie physique et d'optique, Université Laval, Québec (Québec), Canada G1V 0A6
2. Centre interdisciplinaire en modélisation mathématique, Université Laval, Québec (Québec), Canada G1V 0A6
3. Department of Mathematics and Statistics, University of Vermont, Burlington, VT 05405, USA
4. Vermont Complex Systems Institute, University of Vermont, Burlington, VT 05405, USA

**Supplementary Methods 1: Metropolis-Hastings sampling** **2**
Random walk . . . 2
Cluster transformations . . . 2
**Supplementary Methods 2: Convergence diagnostics** **5**
**Supplementary Note 1: Computational complexity** **7**
**Supplementary Note 2: Relationship between $\mathbb{S}^1$ and $\mathbb{H}^2$ models** **9**
**Supplementary Note 3: Differentiable $\mathbb{S}^1$ model** **10**
**Supplementary Note 4: Numerical values of Figure 7** **11**
**Supplementary Note 5: AUC ROC of link prediction** **13**
**Supplementary References** **14**

# Supplementary Methods 1: Metropolis-Hastings sampling

The Metropolis-Hastings algorithm generates Markov chains with arbitrary target invariant measures by (i) sampling transitions between states from a proposal distribution and (ii) accepting or rejecting new states with a carefully crafted acceptance probability. More specifically, the acceptance probability of new state $x^*$ given the previous state $x$ for a continuous random variable is

$$\alpha(x^*, x) = \frac{p(x^*)q(x|x^*)}{p(x)q(x^*|x)}, \tag{1}$$

where $q(y^*|y)$ is the density of the transition kernel, that is, the density of sampling new state $y^*$ from state $y$. In this section, the target $p$ is always the posterior distribution of the Bayesian model.

As explained in the text, we define a global transition kernel, which selects sub-kernels randomly, proportional to their weight: 0.4 for a random walk and 0.2 for each cluster transformation (*flip*, *exchange*, *translate*; see the main text and Fig. 4. We will design all sub-kernels with the target $p$ as their stationary measures, meaning that the proposed state of a subkernel can be accepted with probability 1. The weights are canceled in the acceptance probability and their sole purpose is to help the chain mixing.

## Random walk

For the Markov chain to be irreducible, the sampling space must be accessible from every neighborhood. This is easily satisfied using a random walk algorithm. In this algorithm, a new state $x^*$ is sampled using a normal distribution centered around the previous state $x$. When the random walk subkernel is selected by the global kernel, the set of parameters to explore—that is $\theta$, $\kappa$ or $\beta$—is chosen randomly with equal probability. The main challenge of a random walk Metropolis-Hastings is tuning the variance of the transition kernel. This becomes increasingly difficult in high dimensions: A large variance leads to most proposals being rejected, and a small variance leaves the chain in the same region, increasing the autocovariance and the mixing time in both cases. Hence, we move vertices without significantly altering their angular ordering.

For uniformly distributed vertices on the circle, the distribution of angular separation between two geometrically adjacent vertices is approximately (because of the periodicity on the circle) the exponential distribution of parameter $2\pi/|V|$ (i.e. it is a Poisson point process when ignoring periodicity). To preserve the angular order of vertices on average, we sample each $\theta_u$ from

$$\Theta_u^* = \theta_u + \varepsilon \mod 2\pi, \quad \varepsilon \sim \mathcal{N}_{[-\pi,\pi)}\left(0, \left(\frac{\pi}{2|V|}\right)^2\right), \tag{2}$$

where $\mathcal{N}_{[-\pi,\pi)}$ is the truncated normal distribution on the interval $[-\pi, \pi)$ and where $x \mod 2\pi$ adjusts $x$ such that it lies in $[-\pi, \pi)$. Since the normal distribution is symmetric, there is no bias induced from this transformation $q(\theta^*|\theta) = q(\theta|\theta^*)$.

The transition kernel for $\kappa$ and $\beta$ is a lower truncated normal kernel

$$x^* \sim \mathcal{N}_{(x_{\min},\infty)}(x, \sigma_x^2), \tag{3}$$

where $x_{\min}$ is the smallest value for the parameter $x$. When applying the random walk onto $\kappa$, each individual $\kappa_u^*$ is independently sampled from Supplementary Equation (3). The normalization for Supplementary Equation (3) cannot be omitted when computing the ratio of $q$ in Supplementary Equation (1) because it depends on $x$. We use $\sigma_\kappa = 0.5$ and $\sigma_\beta = 0.3$ to avoid large random walk steps, since large variations would cause too large fluctuations in the connection probabilities. We use $\kappa_{\min} = \epsilon$, $\beta_{\min} = 1$ for consistency with the priors.

## Cluster transformations

For given angular positions $\theta$, we partition the vertices into clusters $\mathcal{C}$ such that every pair of angularly adjacent $\theta_i$ and $\theta_j$ in the same cluster has an angular separation $\Delta(\theta_i, \theta_j)$ below a threshold $t$. The two geometric neighbors of a vertex are the closest vertices in the clockwise and counter-clockwise direction of the circle. The partition of the vertex set is converted to a partition of the circle by defining the boundaries of clusters as the midpoints between each cluster's endpoints.

Because the cluster transformations are discrete, we define a subkernel's probability *mass* function $Q[\Theta^* = \theta^*|\theta]$, which gives the probability of sampling a new set of positions $\theta^*$ when the coordinates are currently equal to $\theta$. For the cluster transformation, the acceptance probability becomes

$$\alpha(\theta^*, \theta) = \frac{p(\theta^*|G)Q[\Theta^* = \theta|\theta^*]}{p(\theta|G)Q[\Theta^* = \theta^*|\theta]}. \tag{4}$$

Each cluster transformation operates on a subset $\Lambda$ of the partition, $\Lambda \subseteq \mathcal{C}$, containing a predetermined number of clusters. For instance, when we apply a translation and move cluster $C_1 \in \mathcal{C}$ to the position of cluster $C_2 \in \mathcal{C}$, then $\Lambda = \{C_1, C_2\}$. Since $\Lambda$ is not ordered, we choose to translate $C_1$ to $C_2$ or $C_2$ to $C_1$ with equal probability: $\mathbb{P}[\Theta^* = \theta^*|\Lambda, \theta] = 1/2$. (This situation does not arise for the *flip* transformation because it involves a single cluster, nor for the *exchange* transformation because it is symmetric.)

The probability $Q$ of sampling the new state is found by marginalizing over all admissible partitions $\mathcal{C}$ (i.e., supersets of $\Lambda$)

$$Q[\Theta^* = \theta^*|\theta] = \sum_{\mathcal{C} \supseteq \Lambda} \mathbb{P}[\Theta^* = \theta^*|\Lambda, \theta]\mathbb{P}[\mathbf{\Lambda} = \Lambda|\theta], \tag{5}$$

where $\mathbb{P}[\mathbf{\Lambda} = \Lambda|\theta]$ is the probability mass function of proposed clusters $\Lambda$ (random variables are typeset in bold to distinguish them from their values). This equation holds if the cluster transformation only yields $\theta^*$ when operating on that specific $\Lambda$. This is the case for our cluster transformations except for very specific $\theta$ that have measure zero.

To define and calculate $\mathbb{P}[\mathbf{\Lambda} = \Lambda|\theta]$, we first note that a partition $\mathcal{C}$ usually contains more clusters than what is strictly required by the transformation, and so we choose $\Lambda$ randomly from $\mathcal{C}$. When there isn't a sufficient number of clusters in the sampled partition $\mathcal{C}$, the proposed $\theta^*$ is automatically rejected. For the sake of simplicity and efficiency, we use a uniform distribution corresponding to

$$\mathbb{P}[\mathbf{\Lambda} = \Lambda|\mathcal{C}, \theta] = \binom{|C|}{|\Lambda|}^{-1}. \tag{6}$$

(We note that targeted cluster selection could be an interesting future research direction.)

Since the hyperbolic space has a hierarchical structure, natural clusters can emerge at different scales, and we found it helpful to use a random threshold $T$ to sample the partitions. This adds a bit of mathematical complexity, as we will now need to think of the cluster proposal probability $\mathbb{P}[\mathbf{\Lambda} = \Lambda|\theta]$ as the marginal of $\mathbb{P}[\mathbf{\Lambda} = \Lambda, \mathcal{C}|\theta]$ over all partitions. To compute this probability, we note that there exists an interval of threshold values $T \in [t, t')$ that yields the same partition $\mathcal{C}$. Since our partitioning algorithm is otherwise deterministic, we can convert the probability of sampling a particular partition $\mathcal{C}$ to the probability of sampling the threshold in that interval,

$$\mathbb{P}[\boldsymbol{\mathcal{C}} = \mathcal{C}|\theta] = \mathbb{P}[T \in [t, t') \mid \theta], \tag{7}$$

where $\boldsymbol{\mathcal{C}}$ is the random variable of the partition. A uniform distribution over $[0, \pi]$ might seem reasonable for $T$, but it turns out to be a poor choice because the density of vertices per radian depends on the number of vertices. In other words, for the same threshold value, increasing the number of vertices would eventually lead us to propose a single cluster with probability close to 1 (unless there are gaps that never contain any vertices).

To take this into consideration, we parameterize the distribution of $T$ using the probability $\xi$ that at least one vertex $u$ is within the separation threshold $t$ of another vertex $v$

$$\xi := \mathbb{P}[\exists u : |\theta_u| < t/2] = 1 - \left(1 - \frac{t}{\pi}\right)^{|V|-1}, \tag{8}$$

where we assume that the angles are uniformly distributed and set $\theta_v = 0$ without loss of generality. By rearranging this equation, we get

$$t(|V|, \xi) = \pi(1 - (1 - \xi)^{1/(|V|-1)}). \tag{9}$$

In the algorithm, we draw $T$, by analogy to the random walk subkernel for the embedding coordinates:

$$T \sim \mathcal{N}_{[0,\pi)}\left(t(|V|, 0.9), \left(\frac{\pi}{2|V|}\right)^2\right). \tag{10}$$

In order to compute Supplementary Equation (5), we need an efficient way to find every partition $\mathcal{C} \supseteq \Lambda$ and another to find the intervals $[t, t')$ of Supplementary Equation (7). Luckily, our partitioning algorithm makes this feasible: A cluster can only shrink as $T$ decreases and can only grow as $T$ increases. This means that given $\Lambda$ and $\theta$, all valid partitions $\mathcal{C} \subseteq \Lambda$ are obtained within an interval $T \in [t_{\min}, t_{\max})$. The values of $t_{\min}(\Lambda)$ and $t_{\max}(\Lambda)$ are the largest in-cluster and the smallest inter-cluster angular separations found for any cluster of $\Lambda$ respectively

$$t_{\min}(\Lambda) = \max_{C_j \in \Lambda} \max_{\substack{u \in C_j \\ v \in \mathcal{A}(u) \cap C_j}} \Delta(\theta_u, \theta_v), \tag{11}$$

$$t_{\max}(\Lambda) = \min_{C_j \in \Lambda} \min_{\substack{u \in C_j \\ v \in \mathcal{A}(u) \setminus C_j}} \Delta(\theta_u, \theta_v), \tag{12}$$

where $\mathcal{A}(u)$ is the set of the two angularly adjacent vertices of $u$. The inner maximum of Supplementary Equation (11) is set to 0 when $C_j$ contains only $u$ and the inner minimum of Supplementary Equation (12) is set to $\pi$ when $C_j$ contains all the vertices (they are ill-defined otherwise).

We now determine the thresholds within $(t_{\min}, t_{\max})$ for which the partition changes, which, here, is when the number of clusters changes. These intermediary thresholds are in fact the angular separations of geometrically adjacent vertices outside the required clusters (noted $\{u \notin \Lambda\}$)

$$\{\Delta(\theta_u, \theta_v) | u \notin \Lambda, v \in \mathcal{A}(u)\} \cap (t_{\min}, t_{\max}). \tag{13}$$

These are used to partition the admissible thresholds

$$[t_{\min}, t_{\max}) = [t_{\min}, t_1) \cup [t_1, t_2) \cup \cdots \cup [t_k, t_{\max}), \tag{14}$$

where $k$ is the number of intermediary thresholds and $t_i$ is the $i$th intermediary threshold in ascending order. Hence, denoting $I(\Lambda)$ the set of these subintervals,

$$\mathbb{P}[\boldsymbol{\Lambda} = \Lambda | \theta] = \sum_{[t,t') \in I(\Lambda)} \mathbb{P}[\boldsymbol{\Lambda} = \Lambda | \mathcal{C}, \theta] \, \mathbb{P}[T \in [t, t') \mid \theta], \tag{15}$$

where, with a slight abuse of notation, we have used the fact $\mathcal{C}$ is the partition obtained for thresholds $T \in [t, t')$.

We note that Supplementary Equation (4) is derived from a detailed balance, and thus requires that $Q[\Theta^* = \theta | \theta^*] > 0$ if and only if $Q[\Theta^* = \theta | \theta] > 0$, meaning that each transformation should be reversed by a single Markov transition. This is always the case for our cluster-based transformations because each one can be undone when they operate on the same $\Lambda$. Our partitioning technique also ensures that $\Lambda$ can be a subset of the partition of the transformed angular coordinates $\theta^*$: each cluster transformation cannot place a vertex closer than $t/2$ to the cluster boundary, which means that there exists an interval of threshold $[t, t + \delta)$ that yields a partition of $\theta^*$ containing obtaining $\Lambda$ for $\theta^*$ ($\delta = 0$ if two vertices exactly have a distance of $t/2$ to a cluster boundary, an event of measure zero).

Finally, it's important to note that the angular separation between vertices and cluster boundaries changes. This means that the intermediary thresholds are not the same for $\theta$ and $\theta^*$ and that the interval $[t_{\min}, t_{\max})$ and the intermediary thresholds for $\theta^*$ must also be computed in $Q[\Theta^* = \theta | \theta]$.

In summary, each cluster-based subkernel transition is done by first sampling $T$ according to Supplementary Equation (10), which gives a partition $\mathcal{C}$ for the current angular coordinates $\theta$. We then sample $\Lambda \subseteq \mathcal{C}$ with $|\Lambda|$ being the required size for the transformation. We apply the cluster transformation with the outcome probabilities $\mathbb{P}[\Theta^* = \theta^* | \Lambda, \theta]$, which yields $\theta^*$. We accept $\theta^*$ as the new state with probability $\alpha(\theta^*, \theta)$ of Supplementary Equation (4). The marginalized probability $Q[\Theta^* = \theta | \theta^*]$ that the sampling drew $\theta^*$ is given by Supplementary Equation (5) (and $Q[\Theta^* = \theta | \theta^*]$ is simply obtained by exchanging $\theta \leftrightarrow \theta^*$ in the equations and by using the $\Lambda$ that was sampled to produce $\theta^*$ in the first place).

# Supplementary Methods 2: Convergence diagnostics

Assessing the quality of an MCMC sampler can be challenging. At the very least, one should verify that (1) the autocovariance of the states decreases with the lag and (2) the stationary distribution is identical no matter the initial state. The former indicates how small the error of Monte Carlo estimators is (by virtue of the Markov chain central limit theorem), and the latter suggests that a Markov chain running long enough will lead to the correct stationary distribution. In this section, we present the effective sample size and the potential scale reduction factor, proxies of these desired properties. We also extend these statistics to random variables on the circle.

The Gelman-Rubin [1] potential scale reduction factor $\hat{R}$ indicates whether or not the different chains "agree" on the typical values of the parameters. Let $(x_1^{(m)}, x_2^{(m)}, \ldots, x_N^{(m)})$ be the $m^{\text{th}}$ Markov chain's state, and for the sake of simplicity, let us assume that we have $M$ chains of equal length $N$. The total chain variance is estimated with the weighted average

$$\widehat{\text{var}}^+ := \frac{N-1}{N} W + \frac{1}{N} B, \tag{16}$$

where $W$ and $B/N$ are, respectively, the within-chain average variance and the between-chain variance

$$W = \frac{1}{M} \sum_{m=1}^{M} s_m^2, \tag{17}$$

$$B = \frac{N}{M-1} \sum_{m=1}^{M} (\bar{x}^{(m)} - \bar{x})^2, \tag{18}$$

and where $s_m^2$ and $\bar{x}^{(m)}$ are the sample variance and sample average

$$s_m^2 = \frac{1}{N-1} \sum_{j=1}^{N} (x_j^{(m)} - \bar{x}^{(m)})^2, \tag{19}$$

$$\bar{x}^{(m)} = \frac{1}{N} \sum_{j=1}^{N} x_j^{(m)}, \tag{20}$$

$$\bar{x} = \frac{1}{M} \sum_{m=1}^{M} \bar{x}^{(m)}. \tag{21}$$

The potential scale reduction factor is then

$$\hat{R} := \sqrt{\frac{\widehat{\text{var}}^+}{W}}. \tag{22}$$

When an MCMC algorithm mixes properly, the chains' $\hat{R} \to 1$ as $N \to \infty$. We use the "split-$\hat{R}$" variant [2], where each chain is split in two for the computation of $\hat{R}$. This adjustment helps detect a within-chain lack of convergence. Note that having a small $\hat{R}$ is a necessary but insufficient convergence condition.

The effective sample size quantifies how many sample points of the sample are considered independent. The (unnormalized) sample autocovariance is

$$a_m(\tau) = \sum_{j=1}^{N-\tau} (x_j^{(m)} - \bar{x}^{(m)})(x_{j+\tau}^{(m)} - \bar{x}^{(m)}). \tag{23}$$

The effective sample size of chain $m$ is [3]

$$n_{\text{eff}}^{(m)} \approx \frac{N}{1 + 2\sum_{\tau=1}^{N} \rho_m(\tau)} \tag{24}$$

where $\rho_m(\tau) = a_m(\tau)/a_m(0)$ is the normalized sample autocovariance. In practice, Supplementary Equation (23) is noisy for large $\tau$ because there are not enough sample points. We use a maximum lag of $\tau = \lfloor N/50 \rfloor$.

Autocovariance can be combined across chains using [4]

$$\rho(\tau) = 1 - \frac{W - \frac{1}{M}\sum_{m=1}^{M} s_m^2 \rho_m(\tau)}{\widehat{\text{var}}^+}, \tag{25}$$

which yields the global effective sample size

$$S_{\text{eff}} \approx \frac{NM}{1 + 2\sum_{\tau=1}^{N} \rho(\tau)}. \tag{26}$$

We use the same heuristic as $n_{\text{eff}}^{(m)}$ for the maximal lag value.

$S_{\text{eff}}$ and $\hat{R}$ statistics are typically used for continuous random variables defined on the real line. Hence, we use these for the parameters $\kappa_u$ and $\beta$. However, they are not appropriate for the angular coordinates because of the cyclic boundary condition. The issue stems from additions and subtractions that appear in averages, Supplementary Equation (26) and Supplementary Equation (22).

To extend $S_{\text{eff}}$ and $\hat{R}$ to a Markov chain realization $(\theta_0^{(m)}, \theta_1^{(m)}, \ldots, \theta_N^{(m)})$ on the circle, we use the circular analogous of the sample average and the sample correlation coefficient, which are respectively [5]

$$\bar{\phi} := \arg\left(\sum_{j=1}^{S} \exp\{i\phi_j\}\right), \tag{27}$$

$$r_{\Phi,\Psi} := \frac{\sum_{j=1}^{S} \sin\left(\phi_j - \bar{\phi}\right) \sin\left(\psi_j - \bar{\psi}\right)}{\sqrt{\sum_{j=1}^{N} \sin^2\left(\phi_j - \bar{\phi}\right)}\sqrt{\sum_{j=1}^{N} \sin^2\left(\psi_j - \bar{\psi}\right)}}, \tag{28}$$

where $i$ is the imaginary number, and $(\phi_j)_{j=1}^{S}$ and $(\psi_j)_{j=1}^{S}$ are i.i.d. samples of $\Phi$ and $\Psi$ respectively with $\Phi$ and $\Psi$ being random variables on the circle. Note that, to simplify notation, $\theta_j$ denotes the $j$th state of the Markov chain realization instead of the angular coordinate of vertex $j$.

The circular autocovariance at lag $\tau$ is obtained directly from Supplementary Equation (28) with the sample points $\phi_j = \theta_j$ and their lagged values $\psi_j = \theta_{j+\tau}$. Since the numerator is analogous to the unnormalized sample covariance, we define the unnormalized sample autovariance

$$a_\circ(\tau) = \sum_{j=1}^{N-\tau} \sin\left(\theta_j - \bar{\theta}\right) \sin\left(\theta_{j+\tau} - \bar{\theta}\right) \tag{29}$$

and the normalized autocovariance function

$$\rho_\circ(\tau) := \frac{a_\circ(\tau)}{a_\circ(0)} \tag{30}$$

that leads to the circular effective sample size

$$n_{\text{eff}}^\circ \approx \frac{1}{1 + 2\sum_{\tau=1}^{N} \rho_\circ(\tau)}. \tag{31}$$

To obtain the circular equivalents of $S_{\text{eff}}$ and $\hat{R}$, we use the circular sample average for $\bar{x}$ and $\bar{x}^{(m)}$ and substitute the subtractions $(\phi - \psi)$ with $\Delta(\phi, \psi)$ in Supplementary Equations (18) and (19).

# Supplementary Note 1: Computational complexity

The main drawback of using MCMC is that it typically scales poorly with the dimension of the sampling space. In the case of the $\mathbb{S}^1$ model, this sampling space consists of $2|V|+1$ parameters: $|V|$ angular coordinates, $|V|$ expected degrees and $\beta$.

The complexity of our particular approach, BIGUE, is as follows. For the random walk described in section Random walk of Supplementary Methods 1, sampling $\Theta^*$ and computing the acceptance probability require $\mathcal{O}(|V|)$ and $\mathcal{O}(|V|^2)$ time, respectively, since the acceptance ratio contains one term for every pair of vertices. This is an unavoidable bottleneck as disconnected vertices contribute greatly to the likelihood in the $\mathbb{S}^1$ model.

For the cluster transformations discussed in section Cluster transformations of Supplementary Methods 1, the calculation of the acceptance probability also consists in a bottleneck. A number of steps have linear complexity in the number of vertices. These include partitioning vertices into clusters $\mathcal{C}$; performing the cluster transformation; and finding the thresholds $t_{\min}$, $t_{\max}$ and $(t_i)_{i=1}^k$. Other steps are quicker. Sampling $t$ and clusters both take $\mathcal{O}(1)$ steps (at most two clusters sampled), and computing the biases induced by ($t_{\min}$, $t_{\max}$, $(t_i)_{i=1}^k$) takes $\mathcal{O}(|\mathcal{C}|)$ time. Computing the posterior density, however, again requires $\mathcal{O}(|V|^2)$ steps.

In summary, both kinds of sampling iterations scale in $\mathcal{O}(|V|^2)$ in time because of the likelihood. While caching partial sums of the log-likelihood could lessen the complexity of cluster moves, it would not provide a significant improvement unless the clusters involve a small number of vertices.

In addition to the quadratic scaling of the iterations, the sampling space volume grows exponentially with the number of variables. This is highlighted in Supplementary Figure 1a where using the same thinning as in Fig. 3d of the main text, the Markov chain states still have a significant autocovariance. Supplementary Figure 1a suggests that having little to no autocovariance between states would require skipping 10 iterations, which corresponds to keeping 1 sample point for every $100,000$ iterations. This is a clear indication of the non-linearity of mixing: sampling a graph with 3.33 times the number of vertices requires 10 times as many iterations.

Nonetheless, the chains settle to embeddings compatible with the ground truth and Mercator, as shown in Supplementary Figure 1b-d. This means we can expect BIGUE to work on larger graphs, but it requires a lot of computing time. With the current implementation of the algorithm, good quality samples for graphs much larger than 100 vertices cannot be obtained in a reasonable time.

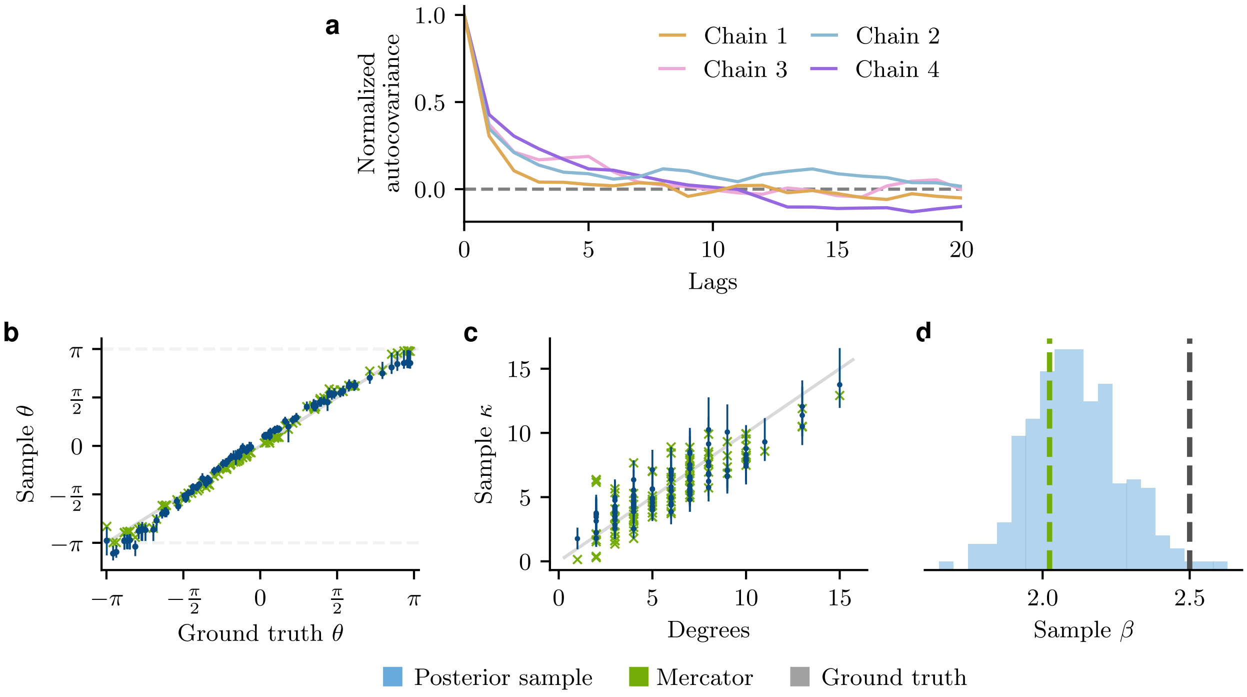


Supplementary Figure 1: Inference for a synthetic graph of 100 vertices. **(a)** Normalized autocovariance of each chain averaged over all parameters at different lags. Posterior estimation of the **(b)** angular coordinates $\theta$ **(c)** parameters $\kappa$ **(d)** inverse temperature $\beta$. In panels (b-d), values obtained from BIGUE, Mercator and the ground truth are displayed in shades of blue, green and gray, respectively. The graph is generated with the same parameters used for the synthetic graph of Fig. 1 of the main text. 400 total embeddings are sampled with four chains with a thinning of $10,000$ iterations. Each chain is initialized without access to ground truth as in Fig.3b and runs for 50 iterations before samples are recorded (warm up or burn-in). The highest potential scale reduction factor for this simulation is $\hat{R}_{\max} = 1.43$, and the effective sample sizes $S_{\text{eff}}$ median is 231.80.

## Supplementary Note 2: Relationship between $\mathbb{S}^1$ and $\mathbb{H}^2$ models

While we developed our algorithm for the $\mathbb{S}^1$ formulation of hyperbolic random graphs, some measures, like the greedy success rate, and visualization such as Fig. 1 of the main text use the hyperbolic coordinates in $\mathbb{H}^2$ embedding. They are formally related by coordinate transformation

$$r_u = R_{\mathbb{H}} - 2\ln\frac{\kappa_u}{\kappa_{\min}} \tag{32}$$

with $R_{\mathbb{H}} = 2\ln\frac{|V|}{\mu\pi\kappa_{\min}}$ where $\kappa_{\min} > 0$ is the smallest allowable $\kappa$ value (we set $\kappa_{\min} = 1$), edge probabilities in the $\mathbb{S}^1$ model can be rewritten as

$$\mathbb{P}[a_{uv} = 1 \mid x, \beta] = \frac{1}{1 + \exp\Big(\beta(r_u + r_v + 2\ln\frac{\Delta(\theta_u,\theta_v)}{2} - R_{\mathbb{H}})\Big)}. \tag{33}$$

We retrieve the hyperbolic random graph model connection probability [6]

$$\mathbb{P}[a_{uv} = 1 \mid x, \beta] = \frac{1}{1 + \exp(\beta(d_{\mathbb{H}}(x_u, x_v) - R_{\mathbb{H}}))} \tag{34}$$

using the following approximation of the hyperbolic distance

$$\begin{aligned} d_{\mathbb{H}}(x_u, x_v) &= \operatorname{arccosh}\Bigg(\cosh(r_u)\cosh(r_v) - \sinh(r_u)\sinh(r_v)\cos(\theta_u - \theta_v)\Bigg), \\ &\approx r_u + r_v + 2\ln\frac{\Delta(\theta_u,\theta_v)}{2}, \end{aligned} \tag{35}$$

where $x_u = (r_u, \theta_u)$ is the position of vertex $u$, and $r_u$ and $\theta_u$ are respectively the radial and angular coordinates in the hyperboloid model.

## Supplementary Note 3: Differentiable $\mathbb{S}^1$ model

As suggested in Fig. 2 of the main text for unconnected vertices, the gradient of the likelihood is undefined when two vertices, $u$ and $v$, have the same angular coordinate $\theta_u = \theta_v$. The culprit is the derivative of $\Delta(\theta_u, \theta_v)$ with respect to $\theta_u$, since the function contains two absolute values. For a given value of $\theta_v$, we have that $-\pi + \theta_v \leq \theta_u < \pi + \theta_v$, which contains at most three discontinuities: $\theta_u = \theta_v$ and $\theta_u - \theta_v \in \{-2\pi, -\pi, \pi, 2\pi\}$. One way to smoothen these sharp transitions is to replace each absolute value with

$$|x| \approx x\left(\frac{2}{1+e^{-bx}} - 1\right) := \tilde{a}(x). \tag{36}$$

This approximation is exact in the limit of $b \to \infty$, which allows us to control the sharpness of the gradient. Beyond the obvious distortions around the discontinuities, another artifact of the approximation is that the rotation symmetry is lost: the gradient doesn't decrease to 0 at $\pm 2\pi$, while it does at $\theta_u = \theta_v$ and $\theta_u - \theta_v = \pm\pi$, where the approximation is used. Further, while $\tilde{a}(0) = 0$, the approximate separation is not zero for $\theta_u = \theta_v$ because $\pi - \tilde{a}(\pi) > 0$.

We found in practice that using $b > 3$ caused gradient divergences in Stan. Supplementary Figure 2 compares the exact angular separation to the approximate one with $b = 3$. While the error seems small, densely connected groups of vertices are usually tightly grouped angularly, which can result in incorrect embeddings.

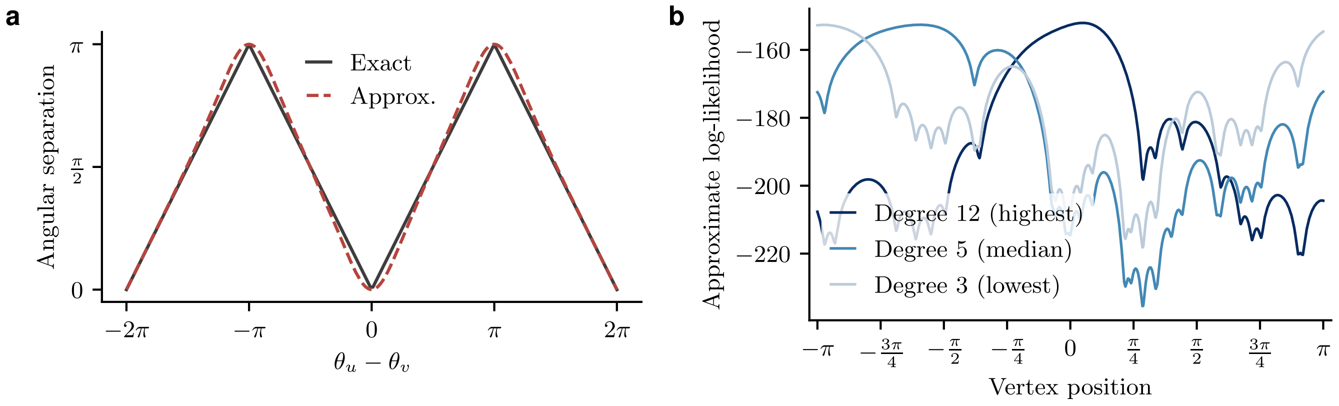


Supplementary Figure 2: **(a)** Differentiable approximation of the angular separation with $b = 3$. **(b)** Figure 2 of the main text using the Differentiable $\mathbb{S}^1$ model with $b = 3$. The approximate angular separation is not invariant to rotations because the gradient doesn't decrease to 0 at $\theta_u = \theta_v$ and at $\theta_u - \theta_v = \pm\pi$. The gradient discontinuities are gone at the cost of distortions of the likelihood.

## Supplementary Note 4: Numerical values of Figure 7

Supplementary Table 1 contains the number of vertices, the effective sample size, the density, the clustering, the shortest path length average and the global hierarchy level with their uncertainty for each dataset of Fig. 7 of the main text.

| Dataset | $\lvert V \rvert$ | $S_{\text{eff}}$ | Density | | | Clustering | | | Shortest path length average | | | Global hierarchy level | |
|---|---|---|---|---|---|---|---|---|---|---|---|---|---|
| | | | Orig. | BIGUE | Mercator | Orig. | BIGUE | Mercator | Orig. | BIGUE | Mercator | BIGUE | Mercator |
| Macaque | 47 | 431 [361, 611] | 0.29, | 0.28 [0.27, 0.29], | 0.29 [0.28, 0.29] | 0.55, | 0.51 [0.50, 0.53], | 0.54 [0.53, 0.55] | 1.85, | 1.83 [1.80, 1.86], | 1.84 [1.81, 1.85] | 0.61 [0.60, 0.64], | 0.63 [—] |
| Zachary | 33 | 933 [705, 1159] | 0.15, | 0.14 [0.13, 0.15], | 0.15 [0.14, 0.15] | 0.26, | 0.30 [0.27, 0.33], | 0.31 [0.30, 0.34] | 2.39, | 2.10 [2.00, 2.20], | 2.30 [2.22, 2.35] | 0.55 [0.51, 0.64], | 0.80 [—] |
| Critics | 29 | 959 [683, 1154] | 0.18, | 0.17 [0.16, 0.18], | 0.13 [0.12, 0.14] | 0.17, | 0.31 [0.28, 0.35], | 0.25 [0.21, 0.28] | 2.28, | 2.11 [1.99, 2.21], | 2.60 [2.44, 2.75] | 0.35 [0.31, 0.42], | 0.62 [—] |
| Gangs | 23 | 1059 [553, 1152] | 0.27, | 0.26 [0.24, 0.27], | 0.27 [0.26, 0.28] | 0.36, | 0.41 [0.39, 0.44], | 0.42 [0.40, 0.44] | 1.77, | 1.80 [1.74, 1.86], | 1.81 [1.77, 1.85] | 0.35 [0.32, 0.43], | 0.58 [—] |
| Zebras | 23 | 645 [385, 806] | 0.42, | 0.41 [0.40, 0.43], | 0.42 [0.41, 0.42] | 0.84, | 0.76 [0.74, 0.80], | 0.85 [0.84, 0.86] | 1.86, | 1.78 [1.70, 1.84], | 1.90 [1.85, 1.91] | 0.32 [0.30, 0.35], | 0.56 [—] |
| Terrorism | 18 | 1048 [759, 1135] | 0.41, | 0.40 [0.37, 0.41], | 0.41 [0.39, 0.41] | 0.56, | 0.55 [0.52, 0.58], | 0.58 [0.57, 0.59] | 1.65, | 1.65 [1.60, 1.70], | 1.65 [1.62, 1.67] | 0.48 [0.45, 0.52], | 0.56 [—] |
| Kangaroo | 16 | 509 [411, 600] | 0.75, | 0.74 [0.72, 0.75], | 0.75 [0.74, 0.75] | 0.85, | 0.84 [0.83, 0.86], | 0.85 [0.85, 0.86] | 1.25, | 1.26 [1.24, 1.27], | 1.25 [1.24, 1.25] | 0.23 [0.20, 0.27], | 0.22 [—] |
| Tribes | 16 | 962 [521, 1125] | 0.48, | 0.46 [0.41, 0.47], | 0.49 [0.47, 0.51] | 0.53, | 0.55 [0.51, 0.59], | 0.56 [0.52, 0.58] | 1.54, | 1.57 [1.49, 1.60], | 1.53 [1.48, 1.55] | 0.28 [0.22, 0.32], | 0.42 [—] |

Supplementary Table 1: Numerical values of the properties shown in Fig. 7 of the main text. For each property, the reported values are in order: original, BIGUE, and Mercator. For the effective sample size $S_{\text{eff}}$, the interquartile range is given instead of the highest density interval. Each sample is a combination of 4 chains of length 300. The effective sample size can be greater than the sample size when the autocovariance is negative on odd lags.

## Supplementary Note 5: AUC ROC of link prediction

A common metric used in binary classification is the receiver operating characteristic curve (ROC). It quantifies the sensitivity of the estimator as a function of the false positive rate. The area under the curve of the AUC (AUC ROC, here shortened as AUC), is a scalar that summarizes this curve: a perfect estimator has an AUC of 1 and a random classification estimator has an AUC of 0.5. The AUC for link prediction is computed using each pair of vertices in the graph.

Supplementary Figure 3a illustrates that Mercator is a better predictor of the original graph than the Bayesian model—this is simply because Mercator finds a embedding with a higher likelihood. After removing 5% of the edges, Mercator's AUC drops but remains higher than that of the Bayesian model. This is not surprising because most edges still exist and removed edges are a small portion of the set of pairs of vertices.

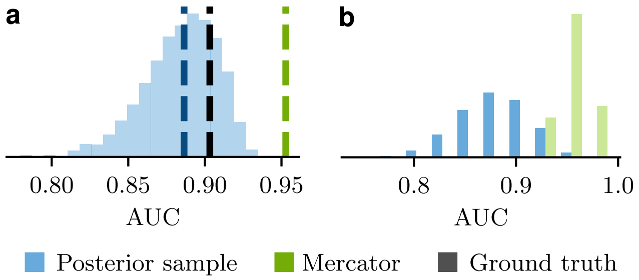


Supplementary Figure 3: Area under the receiver operating characteristic curve (AUC) for **(a)** the synthetic graph of Fig. 1 **(b)** the synthetic graphs where 5% of the edges were removed. The blue dotted line in panel (a) is the median of the posterior sample.

## Supplementary References


[1] A. Gelman and D. B. Rubin, Statist. Sci. **7**, 457 (1992).

[2] A. Gelman, J. B. Carlin, H. S. Stern, D. B. Dunson, A. Vehtari, and D. B. Rubin, *Bayesian Data Analysis*, 3rd ed. (CRC Press, 2013).

[3] A. Sokal, in *Functional Integration*, edited by C. DeWitt-Morette, P. Cartier, and A. Folacci (Springer US, 1997) pp. 131–192.

[4] A. Vehtari, A. Gelman, D. Simpson, B. Carpenter, and P.-C. Bürkner, Bayesian Anal. **16**, 667 (2021).

[5] S. R. Jammalamadaka and A. Sengupta, *Topics In Circular Statistics* (World Scientific Publishing, 2001).

[6] D. Krioukov, F. Papadopoulos, M. Kitsak, A. Vahdat, and M. Boguñá, Phys. Rev. E **82**, 036106 (2010).
